# Supplementary material for: Incorporating Explicit Uncertainty Estimates into Deep Offline Reinforcement Learning
Source: arXiv:2206.01085 source file (2022-06-02)
Supplement: Supplementary file 1 [file appendix.tex]

\onecolumn
\appendix
\section*{Appendix}

\section{Scaling of \xorls}\label{app:scaling}

\begin{figure*}[h]
    \centering
    
    \begin{subfigure}{\linewidth}
		\centering
		\includegraphics[width=0.9\linewidth]{figs/ds_size.pdf}\\
    \cblock{52}{138}{189}\hspace{1mm}Random\hspace{1.5mm}
    \cblock{166}{6}{40}\hspace{1mm}ICM\hspace{1.5mm}
    \cblock{122}{104}{166}\hspace{1mm}Disagreement\hspace{1.5mm}
    \cblock{70}{120}{33}\hspace{1mm}RND\hspace{1.5mm}
    \cblock{213}{94}{0}\hspace{1mm}Proto\hspace{1.5mm}
    \cblock{204}{121}{167}\hspace{1mm}APT\hspace{1.5mm}
    \cblock{86}{180}{233}\hspace{1mm}APS\hspace{1.5mm}
    \cblock{0}{158}{115}\hspace{1mm}DIAYN\hspace{1.5mm}
    \cblock{240}{228}{66}\hspace{1mm}SMM
    \caption{Correlation between TD3 performance and the unsupervised data collection transition budget.}
        \label{fig:ds_size_data}
     \end{subfigure}
     		
  \begin{subfigure}{\linewidth}
		\centering
		\includegraphics[width=0.9\linewidth]{figs/ds_size_eval.pdf}\\
		\cblock{52}{138}{189}\hspace{1mm}BC\hspace{1.5mm}
    \cblock{213}{94}{0}\hspace{1mm}TD3+BC\hspace{1.5mm}
    \cblock{122}{104}{166}\hspace{1mm}CRR\hspace{1.5mm}
    \cblock{70}{120}{33}\hspace{1mm}CQL\hspace{1.5mm}
    \cblock{166}{6}{40}\hspace{1mm}TD3\hspace{1.5mm}
		\caption{Correlation between performance of various offline RL algorithms and unsupervised data collection transition budget for ICM. }
        \label{fig:ds_size_eval}
     \end{subfigure}

	\caption{Testing the impact of the size of unsupervised data collection budget on downstream offline RL performance.~\cref{fig:ds_size_data} provides a breakdown by datasets, while~\cref{fig:ds_size_eval} provides a breakdown by offline RL algorithms. Generally, larger datasets demonstrate better performance across both exploration and offline RL algorithms.}
	%however, in some cases (i.e. Walker Run) current URL agents are unable to produce datasets that can match online RL performance.  }
        \label{fig:ds_size}
  
     \vspace{-0.5cm}
\end{figure*}

\textbf{Q5}: How effective is~\xorls~as we scale the data collection budget?
\textbf{A1:} \textit{In general, all algorithms see improved performance with increased data collection budget}.

To confirm, this we collect datasets in the Walker domain with data collection budgets ranging from 100k to 10M transitions (100 to 10k episodes) using all nine unsupervised data collection algorithms. We then run offline RL on these datasets for two different rewards: Walk and Run. To compare the different datasets we run offline TD3 on each (since TD3 was the strongest performer in prior experiments). Then to compare the offline RL algorithms, we run each of our five offline RL algorithms on the datasets generated by ICM (since ICM was the strongest performing dataset with TD3). Results are in \cref{fig:ds_size}.

First, we evaluate the results across the different exploration algorithms. All algorithms see returns to scale, but we do observe gains beginning to saturate by 10M transitions on the Run task before reaching optimal performance suggesting there is still room for improved algorithms. In low-data settings we see the best performance from DIAYN while in the high-data regime ICM begins to dominate. We note that the random agent also sees return to scale, suggesting that the Walk task is not a difficult exploration problem.

We can also compare across the different offline RL algorithms on the ICM data. Again we see clear returns to scale as performance improves with dataset size. As in previous experiments we see that TD3 is the strongest algorithm and this holds true across dataset sizes.

\section{Hyper-parameters}
\label{app:hyperparams}
In this section we comprehensively describe configuration of both unsupervised RL and offline RL algorithms.
\subsection{Unsupervised RL Hyper-parameters}
We adhere closely to the parameter settings from URLB~\citep{laskin2021urlb}. We list the common hyper-parameters in~\cref{table:url_common_hp} and per-algorithm hyper-parameters in~\cref{table:url_individual_hp}. 

\begin{table}[h!]
\caption{\label{table:url_common_hp} Common hyper-parameters for unsupervised RL algorithms.}
\centering
\begin{tabular}{lc}
\hline
Common hyper-parameter       & Value \\
\hline
\: Replay buffer capacity & $10^6$ \\
\: Seed frames & $4000$ \\
\: Mini-batch size & $1024$ \\
\: Discount ($\gamma$) & $0.99$ \\
\: Optimizer & Adam \\
\: Learning rate & $10^{-4}$ \\
\: Agent update frequency & $2$ \\
\: Critic target EMA rate ($\tau_Q$) & $0.01$ \\
\: Hidden dim. & $1024$ \\
\: Exploration stddev clip & $0.3$ \\
\: Exploration stddev value & $0.2$ \\

\hline
\end{tabular}

\end{table}

\begin{table}[h!]
\caption{\label{table:url_individual_hp} Individual hyper-parameters for unsupervised RL algorithms.}
\centering
\begin{tabular}{lc}
\hline
Random hyper-parameter       & Value \\
\hline
\: Policy distribution & $\mathrm{uniform}$ \\
\hline
ICM hyper-parameter       & Value \\
\hline
\: Reward transformation & $\log (r + 1.0)$ \\
\: Forward net arch. & $(|\mathcal{O}| + |\mathcal{A}|) \to 1024 \to 1024 \to |\mathcal{O}|$ $\textrm{ReLU}$ MLP\\
\: Inverse net arch. & $(2 \times |\mathcal{O}|) \to 1024 \to 1024 \to |\mathcal{A}|$ $\textrm{ReLU}$ MLP\\
\hline
Disagreement hyper-parameter       & Value \\
\hline
\: Ensemble size & $5$ \\
\: Forward net arch: & $(|\mathcal{O}| + |\mathcal{A}|) \to 1024 \to 1024 \to |\mathcal{O}|$ $\textrm{ReLU}$ MLP\\
\hline
RND hyper-parameter       & Value \\
\hline
\: Predictor \& target net arch. & $|\mathcal{O}| \to 1024 \to 1024 \to 512$ $\textrm{ReLU}$ MLP\\
\: Normalized observation clipping & 5 \\
\hline
APT hyper-parameter       & Value \\
\hline
\: Reward transformation & $\log (r + 1.0)$ \\
\: Forward net arch. & $(512 + |\mathcal{A}|) \to 1024 \to 512$ $\textrm{ReLU}$ MLP\\
\: Inverse net arch. & $(2 \times 512) \to 1024 \to |\mathcal{A}|$ $\textrm{ReLU}$ MLP\\
\: $k$ in $\mathrm{NN}$ & $12$ \\
\: Avg top $k$ in $\mathrm{NN}$ & True \\
\hline
Proto hyper-parameter       & Value \\
\hline
\: Predictor dim. & $128$ \\
\: Projector dim. & $512$ \\ 
\: Number of prototypes & $512$ \\
\: Softmax temperature & $0.1$ \\
\: $k$ in $\mathrm{NN}$ & $3$ \\
\: Number of candidates per prototype & $4$ \\
\: Encoder target EMA rate ($\tau_\mathrm{enc}$) & $0.05$ \\
%\: Intrinsic reward coefficient ($\alpha$) & $0.2$ \\
\hline
SMM hyper-parameter & Value \\
\hline 
\: Skill dim. & $4$ \\
\: Skill discriminator learning rate & $10^{-3}$ \\
\: VAE lr & $10^{-2}$ \\

\hline
DIAYN hyper-parameter       & Value \\
\hline

\: Skill dim & 16 \\ 
\: Skill sampling frequency (steps) & 50 \\
\: Discriminator net arch. & $512 \to 1024 \to 1024 \to 16$ $\textrm{ReLU}$ MLP  \\
\hline 
APS hyper-parameter       & Value \\
\hline
\: Reward transformation & $\log (r + 1.0)$ \\
\: Successor feature dim. & $10$ \\
\: Successor feature net arch. & $|\mathcal{O}| \to 1024 \to 1024 \to 10$ $\textrm{ReLU}$ MLP\\
\: $k$ in $\mathrm{NN}$ & $12$ \\
\: Avg top $k$ in $\mathrm{NN}$ & True \\
\: Least square batch size & $4096$ \\
\hline

\end{tabular}

\end{table}

\clearpage

\subsection{Offline RL Hyper-parameters}
In~\cref{table:orl_common_hp} we present a common set of hyper-parameters used in our experiments, while in~\cref{table:orl_individual_hp}
we list individual hyper-parameters for each method. To select hyper-parameters for offline RL algorithms we started with from the original hyper-parameters presented in the corresponding papers. We then performed a grid search over the most important parameters (i.e. learning rate, $\alpha$, mini-batch size, etc.) on a supervised dataset collected by TD3~\citep{fujimoto2018addressing} on Cheetah Run. 
\paragraph{TD3+BC} We swept over learning rate $[10^{-3}, 3\cdot10^{-4}, 10^{-4}]$, mini-batch size $[256, 512, 1024]$ and $\alpha$ $[0.01, 0.1, 1.0, 2.5, 5.0, 10.0, 50.0]$. We also found it useful to increase the dimension of hidden layers to $1024$. 
\paragraph{CRR} We swept over the transformation function (indicator, exponent, identity), the number of samples to estimate value function $[5, 10, 20]$ as well as learning rate $[10^{-3}, 3\cdot10^{-4}, 10^{-4}]$ and mini-batch size $[256, 512, 1024]$.
\paragraph{CQL} We swept over $\alpha$ $[0.01, 0.1, 0.5, 1.0, 2.0, 5.0, 10.0]$, the number of sampled actions $[3, 5, 10, 20]$, learning rate $[10^{-3}, 3\cdot10^{-4}, 10^{-4}]$ and mini-batch size $[256, 512, 1024]$.

\begin{table}[h]
\caption{\label{table:orl_common_hp} Common hyper-parameters for offline RL algorithms.}
\centering
\begin{tabular}{lc}
\hline
Common hyper-parameter       & Value \\
\hline
\: Replay buffer capacity & $10^6$ \\
\: Mini-batch size & $1024$ \\
\: Discount ($\gamma$) & $0.99$ \\
\: Optimizer & Adam \\
\: Learning rate & $10^{-4}$ \\
\: Agent update frequency & $2$ \\
\: Training steps & $5\times 10^5$ \\
\hline
\end{tabular}

\end{table}

\begin{table}[h]
\caption{\label{table:orl_individual_hp} Individual hyper-parameters for offline RL algorithms.}
\centering
\begin{tabular}{lc}
\hline
BC hyper-parameter       & Value \\
\hline
\: Num hidden layers & $2$ \\ 
\: Hidden dim. & $1024$ \\
\hline
TD3+BC hyper-parameter       & Value \\
\hline
\: $\alpha$ &$2.5$ \\
\: Critic target EMA rate ($\tau_Q$) & $0.01$ \\
\: Num hidden layers & $2$ \\ 
\: Hidden dim. & $1024$ \\
\hline
CRR hyper-parameter       & Value \\
\hline
\: Num samples to estimate $V$ & $10$ \\ \: Critic target EMA rate ($\tau_Q$) & $0.01$ \\
\: Transformation & indicator \\ 
\: Num hidden layers & $2$ \\ 
\: Hidden dim. & $1024$ \\
\hline
CQL hyper-parameter       & Value \\
\hline
\: $\alpha$ & $0.01$ \\ 
\: Critic target EMA rate ($\tau_Q$) & $0.01$ \\
\: Lagrange & False \\ 
\: Num sampled actions & $3$ \\ 
\: Num hidden layers & $2$ \\ 
\: Hidden dim. & $1024$ \\
\hline
TD3 hyper-parameter       & Value \\
\hline
\: Stddev clip & $0.3$ \\
\: Critic target EMA rate ($\tau_Q$) & $0.01$ \\
\: Num hidden layers & $2$ \\ 
\: Hidden dim. & $1024$ \\
\hline

\end{tabular}

\end{table}
\clearpage
\newpage

\section{Full Results on the PointMass Experiment}
\label{section:app_pm_full_results}

\begin{figure*}[h]
   % \centering

		\centering
		\includegraphics[width=\linewidth]{figs/pm_eval_full.pdf}
		\hspace{1.5mm}
    \cblock{52}{138}{189}\hspace{1mm}Random\hspace{1.5mm}
    \cblock{166}{6}{40}\hspace{1mm}ICM\hspace{1.5mm}
    \cblock{122}{104}{166}\hspace{1mm}Disagreement\hspace{1.5mm}
    \cblock{70}{120}{33}\hspace{1mm}RND\hspace{1.5mm}
    \cblock{213}{94}{0}\hspace{1mm}Proto\hspace{1.5mm}
    \cblock{204}{121}{167}\hspace{1mm}APT\hspace{1.5mm}
    \cblock{86}{180}{233}\hspace{1mm}APS\hspace{1.5mm}
    \cblock{0}{158}{115}\hspace{1mm}DIAYN\hspace{1.5mm}
    \cblock{240}{228}{66}\hspace{1mm}SMM

        \label{fig:pm_eval_full}

    \caption{ Extended figures from~\cref{fig:pm}. }

    % \vspace{-10pt}
\end{figure*}

\newpage

\section{Full Results on Singletask Settings}
\label{section:mult_env_full}

\begin{figure*}[h]
   % \centering

		\centering
		\includegraphics[width=\linewidth]{figs/main_full.pdf}
		\hspace{1.5mm}
    \cblock{52}{138}{189}\hspace{1mm}Random\hspace{1.5mm}
    \cblock{166}{6}{40}\hspace{1mm}ICM\hspace{1.5mm}
    \cblock{122}{104}{166}\hspace{1mm}Disagreement\hspace{1.5mm}
    \cblock{70}{120}{33}\hspace{1mm}RND\hspace{1.5mm}
    \cblock{213}{94}{0}\hspace{1mm}Proto\hspace{1.5mm}
    \cblock{204}{121}{167}\hspace{1mm}APT\hspace{1.5mm}
    \cblock{86}{180}{233}\hspace{1mm}APS\hspace{1.5mm}
    \cblock{0}{158}{115}\hspace{1mm}DIAYN\hspace{1.5mm}
    \cblock{240}{228}{66}\hspace{1mm}SMM

        \label{fig:mult_env_full}

    \caption{Offline evaluation of unsupervised datasets on one task for each of three different domains. Here we choose four representative unsupervised exploration algorithms. }

    % \vspace{-10pt}
\end{figure*}

\newpage

\section{Full Results on Multitask Settings}
\label{section:mult_task_full}

\begin{figure*}[h]
   % \centering

		\centering
		\includegraphics[width=\linewidth]{figs/mt_full.pdf}
		\hspace{1.5mm}
    \cblock{52}{138}{189}\hspace{1mm}Random\hspace{1.5mm}
    \cblock{166}{6}{40}\hspace{1mm}ICM\hspace{1.5mm}
    \cblock{122}{104}{166}\hspace{1mm}Disagreement\hspace{1.5mm}
    \cblock{70}{120}{33}\hspace{1mm}RND\hspace{1.5mm}
    \cblock{213}{94}{0}\hspace{1mm}Proto\hspace{1.5mm}
    \cblock{204}{121}{167}\hspace{1mm}APT\hspace{1.5mm}
    \cblock{86}{180}{233}\hspace{1mm}APS\hspace{1.5mm}
    \cblock{0}{158}{115}\hspace{1mm}DIAYN\hspace{1.5mm}
    \cblock{240}{228}{66}\hspace{1mm}SMM

        \label{fig:mult_task_full}

    \caption{ Offline evaluation of datasets for the Walker environment under three different rewards (Stand, Walk, and Run). We observe that ExORL allows for data relabeling to enable multi-task offline RL. }

    % \vspace{-10pt}
\end{figure*}

\newpage

\section{Offline RL on Suffixes of Unsupervised Datasets}
\label{section:suffix}
In~\cref{fig:suffix} we demonstrate that it is important to use the entire replay buffers collected by~\xorls, rather than only training on the later parts of this data.

\begin{figure*}[h]
    \centering

    \includegraphics[width=0.9\linewidth]{figs/suffix.pdf}\\
        \hspace{1.5mm} \cblock{52}{138}{189}\hspace{1mm}BC\hspace{1.5mm}
    \cblock{166}{6}{40}\hspace{1mm}TD3+BC\hspace{1.5mm}
    \cblock{122}{104}{166}\hspace{1mm}TD3\hspace{1.5mm}
    
    \caption{Instad of training on the full replay buffer collected by ICM, we perform offline RL training on various suffixes of the replay buffer. The x-axis represents segments of the replay buffuer. We observe that it is important to keep around early transitions.}
    \label{fig:suffix}
    % \vspace{-10pt}
\end{figure*}

\newpage
\section{Compute Resources}
\label{app:compute}

\xorls~is designed to be accessible to the RL research community. We provide an efficient implementation of our framework, including data collection, relabeling, and offline RL evaluation, that requires a single GPU. For local debugging experiments we used NVIDIA RTX GPUs. For large-scale runs used to generate all results in this manuscripts, we used NVIDIA Tesla V100 GPU instances. All experiments were run on internal clusters. Each offline RL algorithm trains in roughly 2 hours for 500k gradient steps on the collected datasets.

\section{The ExORL Environments and Tasks}
\label{app:dmc_tasks}
We provide a summary of used environments and tasks in our paper in~\cref{table:benchamrks}.

\begin{table}[!h]
\centering
\begin{tabular}{lccccc}
\hline
Environment & Task & Traits  &$\mathrm{dim}(\mathcal{S})$ & $\mathrm{dim}(\mathcal{A})$   \\

\hline
Walker & Stand & dense reward, easy exploration, locomotion   & $18$ & $6$  \\
 & Walk & dense reward, medium exploration, locomotion   & $18$ & $6$  \\
  & Run & dense reward, hard exploration locomotion   & $18$ & $6$  \\
   & Flip & dense reward, medium exploration, locomotion   & $18$ & $6$  \\

\hline

Cheetah & Run & dense reward, hard exploration, locomotion   & $24$ & $6$  \\
 & Run Backward & dense reward, hard exploration, hard transfer   & $24$ & $6$  \\
\hline

\hline
PointMass Maze & Reach Top Left & sparse reward, hard exploration, hard transfer   & $4$ & $2$  \\

 & Reach Top Right & sparse reward, hard exploration, hard transfer    & $4$ & $2$  \\
  & Reach Bottom Left & sparse reward, hard exploration, hard transfer    & $4$ & $2$  \\
   & Reach Bottom Right & sparse reward, hard exploration, hard transfer    & $4$ & $2$  \\

\hline

Jaco & Reach & sparse reward, hard exploration, manipulation   & $55$ & $6$  \\
\hline

 Cartpole & Swingup  & dense reward, easy exploration   & $4$ & $1$  \\
\hline

\hline
\end{tabular}
\caption{\label{table:benchamrks} A detailed description of used environments and tasks from the DeepMind control suite~\citep{tassa2018deepmind}.}
\end{table}
